# Supplementary material for: Deformable ProtoPNet: An Interpretable Image Classifier Using Deformable Prototypes
Source: arXiv:2111.15000 source file (2024-05-02)

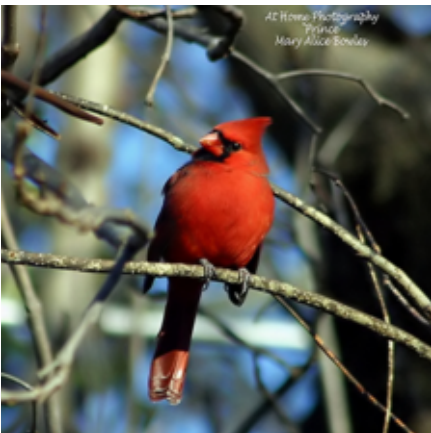

Cardinal

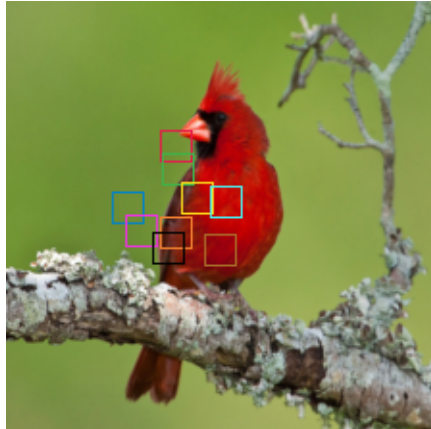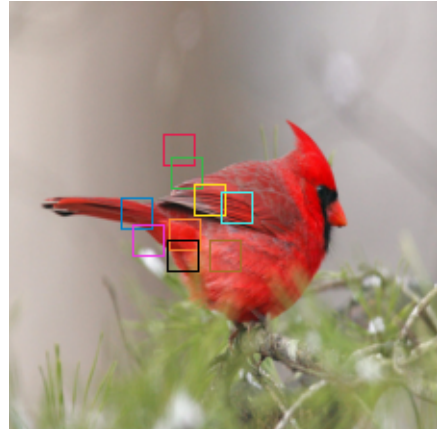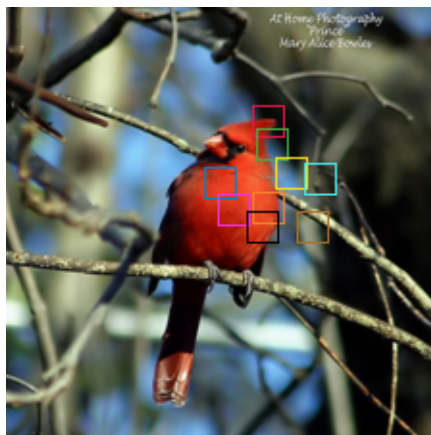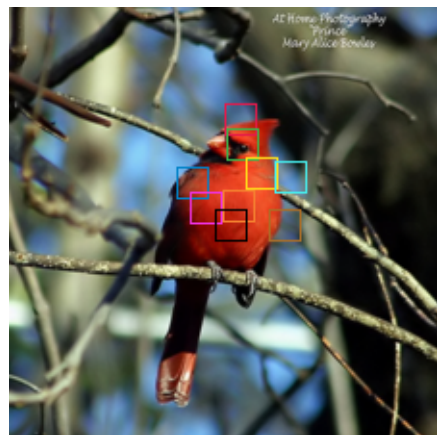

Supplement: Supplementary file 1 [file local_analysis_birds_00003.pdf]
